# Supplementary material for: Impact on clinical guideline adherence of Orient-COVID, a CDSS based on dynamic medical decision trees for COVID19 management: a randomized simulation trial
Source: arXiv:2407.11205 source file (2024-06-21)
Supplement: Supplementary file 1 [file article2_supplement1.pdf]

# Clinical reasoning study

**Please sign the consent to start**

# Case 1

# Scenario:

- Patient, 49 YO, arrived to ER for dyspnea, exacerbating cough and fever. He has also diarrhea and decreased PO intake. He was diagnosed for Covid 9 days ago with a positive PCR. He started a treatment by azithromycin 250 mg daily + levofloxacin 500 mg daily & vitamins C & D.
- In his past medical history, he is known to have high blood pressure treated by fludex, nebilet & coveram.
- At ER, he is conscious with a normal clinical exam unless some crackles heard bilaterally. His vital signs are: BP: 127/70 mmHg; pulse: 111/min; RR 22/min; SpO2 93%; T 36°C

**1- What do you do?**

# Results

- **EKG** Normal
- **ABG**: pH 7.47/ PO2 70/ PCO2 40/ bicar 29/ Sat 93%
- **CT chest**:
  - Plages de condensation parenchymateuse, prenant par endroit un aspect en bande, de topographie à prédominance périphérique et lobaire inférieure bilatérale, montrant par endroit des bronchogrammes aériens notamment le segment apical du lobe inférieur droit, et par endroits une densité en verre dépoli, évoquant une infection au co-vid 19 en phase déjà avancée. L'atteinte parenchymateuse avoisine les 30%.
- **Blood test**:
  - CBC: Hb 14/Ht41/ WBC 2400 (67/23)/ plt 209,000
  - Creat 1.04
  - Na 136/ K 3.15/ Cl 95
  - CRP 48
  - LDH 376
  - Trop Neg
  - D dimers 214
  - IL-6 78 (N < 7)

**2- Do you hospitalize him?**

**If yes, Ward or ICU?**

**3- What treatment will you prescribe for him?**

## **Treatment:**

Oxygen nasal canula 5L/min & Rocephin 2g IV OD And steroids

**4- How do you monitor him?**

## **Monitoring:**

Sat > 95% with tapering well tolerated until O2 stopped

No more fever/ good clinical / Amelioration of blood tests: IL  
6 normal & CRP reduced by 50%

**4- What is your plan now after 48h of  
monitoring?**

# Case 2

# Scenario:

- Patient male, 78 YO, arrived to ER for severe abdominal pain, dyspnea & fever. He was operated of colectomy 10 days ago & he is known to have gastric cancer under chemotherapy.
- In his past medical history, nothing to be mentioned.
- At ER, he is conscious, cachectic, dyspneic with a soft abdomen & diffuse crackles. His vital signs are: BP: 110/80 mmHg; pulse: 98/min; RR 18/min; SpO2 96%; T 37°C. PCR positive

**1- What do you do?**

# Results

- **EKG**: normal
- **Chest CT**:
  - Small bilateral pleural effusion is present larger on the right side.
  - Minimal pericardial effusion is also present.
  - There is a newly developed diffuse bilateral smooth interlobular septal thickening involving the upper and lower lobes.
  - Small peripheral nodules are present. The largest in the left lower lobe. Measures 9 mm.
  - Faint lobular peripheral ground glass opacities are present bilaterally.
  - The findings are atypical for viral pneumonia.
- **Blood test**:
  - CBC: Hb 13.4/Ht 42.2/ WBC 8100 (70/18)/ plt 306,000
  - Creat 1.1
  - Na 141/ K 4.62/ Cl 105
  - CRP 118
  - LDH 250
  - Ferritine 346
  - Trop slightly positive
  - D dimers 1265
  - IL-6 31 (N < 7)

**2- Do you hospitalize him?**

**If yes, Ward or ICU?**

**3- What treatment will you prescribe for him?**

## **Treatment:**

Tazocin 4.5 gIV/6h, Zithromax 250 mg OD, doxiquine 200 mg PO BID, Vit C,D, Zinc, Arixtra 2.5 mg OD

**4- How do you monitor him?**

## **Monitoring:**

Patient always complaining of dyspnea.

Stabilization on floor.

RRT: Severe dyspnea refractory to intervention

**4- What is your plan now after 48h of monitoring?**

# Case 3

# Scenario:

- Patient male, 83 YO, arrived to ER for altered general status, fatigue, diarrhea & melena. He was diagnosed covid positive 5 days ago & started oral treatment by vitamins, hydroxychloroquine & levofloxacin.
- In his past medical history, he is known to have diabetes, high blood pressure, CKD & rheumatoid arthritis. His chronic treatment is: Calcium, Predicor 5 mg OD, omnic 0.4 mg OD, glucovance 500/5 mg OD, adenuric 40 mg OD, xatral 10 mg OD, aspirine 100 mg OD.
- At ER, he is conscious with bilateral basal crackles & soft abdomen. His vital signs are: BP: 118/56 mmHg; pulse: 66/min; RR 18/min; SpO2 92%; T 37°C.

1. What do you do?

# Results

- **EKG**: normal
- **Chest CT**:
  - Parenchymal consolidation affecting most of the posterior region of the lower lobes and the posterior segment of the right upper lobe.
  - Small left pleural effusion.
  - Few patchy ground-glass infiltrates scattered bilaterally.
  - Findings are suggestive of added bacterial infection, aspiration pneumonia should be considered as well.
  - Heart at the upper limit of normal size.
  - No enlarged mediastinal or hilar lymph nodes.
- **Blood test**:
  - CBC: Hb 12.3/Ht 38.6/ WBC 16000 (92/3)/ plt 94,000
  - Creat 6.7
  - Na 138/ K 2.41/ Cl 99
  - CRP 90
  - LDH 290
  - Ferritine 620
  - Trop 195
  - Ddimers 1900
  - IL-6 178 (N < 7)

**2- Do you hospitalize him?**

**If yes, Ward or ICU?**

**3- What treatment will you prescribe for him?**

## Treatment:

Tazocin 2.25 gIV/8h, Zithromax 250 mg OD, dolquine 200 mg PO BID, Viscoflu, mucosolvan, Solumedrol, Oxygen NC 7L/min

**4- How do you monitor him?**

## **Monitoring:**

Gastrosocopy: no bleeding

Correction of electrolyte imbalance & acidosis

CRP & creat reduced

Patient stable hemodynamically

Less oxygen needed

**4- What is your plan now after 48h of monitoring?**

# Case 4

# Scenario:

- Patient female, 68 YO, presented to ER for dyspnea exacerbated in the last 2 days, PCR positive 4 days ago. She is known to have blood hypertension, diabetes, hypercholesterolemia & myelodysplastic syndrome. Her chronic treatment is: Cynt 0.3 BID, Exforge 160/10 OD, cardular 4mg BID, Bisoprolol 5 mg OD, GalvusMet 50/1000 mg BID, Nexium 40 OD, Acifer OD, singulair OD, Ryzodeg & lexotanil 3 mg OD.
- At ER, she is conscious but dyspneic with diffuse wheezing. Her vital signs are: BP: 177/82 mmHg; pulse: 82/min; RR ? /min; SpO2 93%; T 37.2°C

1. What do you do?

# Results

- **EKG**: normal
- **Chest CT**:
  - The main pulmonary artery is mildly dilated measuring 3.2 cm with enlargement of the right and left main pulmonary arteries and interlobar arteries. The findings are compatible with pulmonary hypertension.
  - The hila are prominent bilaterally, most likely due to enlarged pulmonary vessels.
  - Small bilateral pleural effusion is present.
  - Diffuse bilateral inter lobar septal thickening is present bilaterally.
  - There is segmental peribronchovascular consolidation in the right lower lobe.
  - Multiple small pleural based opacities are present. As well as few areas of faint ground-glass opacities.
- **Blood test**:
  - PCR positive (CT 15)
  - CBC: Hb 8.7/Ht 27.1/ WBC 5300 (69/21)/ plt 208,000
  - Creat 0.57
  - Na 136/ K 5.95/ Cl 104
  - CRP 20
  - LDH 223
  - Trop 10.7
  - Ddimers 1103
  - IL-6 28.7 (N < 7)

**2- Do you hospitalize her?**

**If yes, Ward or ICU?**

**3- What treatment will you prescribe for her?**

## Treatment:

Hydroxychloroquine 200 mg BID, Rocephin 1g IV OD,  
Zithromax 250 mg OD, Atrovent Neb TID, Lasix 40 mg BID  
& lovenox 40 mg OD + Oxygen NC 7L/min

**4- How do you monitor her?**

## **Monitoring:**

Good tapering of O<sub>2</sub>

No fever

Clinically stable

Amelioration of blood tests: CRP reduced & Il-6 to 1 & crp to 9.

**4- What is your plan now after 48h of monitoring?**

# Case 5

# Scenario:

- Patient male, 72 YO, presented to ER for weakness, cough, dyspnea, yellow sputum, fever, chills & abdominal pain without diarrhea. Symptoms started 10 days ago. He was treated by augmentin, leflumax & oradus beta without improving.
- He is known to have CLL treated by chemotherapy, diabetes & hypertension. His chronic treatment consists of: Lyrica 75 BID, losanet forte ½ tablet OD & concor 2.5 mg OD.
- He is conscious & well oriented with a normal clinical exam unless abdomindal distension. His vital signs are: BP: 93/52 mmHg; pulse: 80/min; RR 22/min; SpO2 92%; T 37.5°C. PCR positive.

# Results

- **EKG**: normal
- **Chest CT**:
  - The heart is enlarged.
  - The pulmonary artery and the ascending aorta are of normal caliber.
  - No enlarged mediastinal or hilar lymph nodes.
  - The vessels are slightly engorged denoting congestion.
  - Minimal left-sided pleural effusion and Bi-basal atelectatic bands.
  - No suspicious mass or nodule.
  - A 9 mm lipoma at the level of the right atrium.
- **Blood test**:
  - CBC: Hb 13.4/Ht40.1/ WBC 3300 (81/10)/ plt 168,000
  - Creat 1.2
  - Na 137/ K 4.09/ Cl 103
  - CRP 76
  - LDH 293
  - Trp 14
  - Ddimers 188
  - Ferritine 759
  - IL-6 56 (N < 7)

**2- Do you hospitalize him?**

**If yes, Ward or ICU?**

**3- What treatment will you prescribe for him?**

## **Treatment:**

Hydroxychloroquine, Tazocine 4.5 g IV / 8h, solumedrol 40 mg IV BID

**4- How do you monitor him?**

## **Monitoring:**

Stable during 48h but not yet ready to be discharged

Oxygen dependant.

**4- What is your plan now after 48h of monitoring?**

# Case 6

# Scenario:

- Patient female, 82 YO, arrived to ER for severe dyspnea & fever. She was operated for hip replacement 1 week ago.
- In her past medical history, she is known to have hypertension, diabetes, chronic heart failure, oesophageal varices, recurrent DVT & Afib. Her home medications are: concor 5 mg OD, lusopress 20 mg OD, Lasix 125 mg TID, Glucophage, cynt 0.4 mg OD & Xarelto 15 mg OD.
- At ER, she is conscious but dyspneic with irregular pulse & diffuse bilateral crackles. Her vital signs are: BP: 138/89 mmHg; pulse: 130/min; RR 32/min; SpO2 92%; T 38.3°C

• DGB positive

1. What do you do?

# Results

- **EKG:** Afib
- **Chest CT:**
  - The heart is enlarged.
  - The thoracic aorta is of normal size.
  - The main pulmonary artery is mildly dilated measuring 3.2 cm.
  - The mediastinal nodes measure less than 10 mm and are of indeterminate pathological significance.
  - There is no pleural effusion.
  - There is diffuse bilateral mixed patchy ground glass opacities and lobular consolidation involving the
    - upper and lower lobes Centrally and peripherally.
    - The parenchymal involvement in the lower
- **Blood test:**
  - CBC: Hb 7.9/Ht 24.3/ WBC 8600 (92/4)/ plt 229,000
  - Creat 1.57
  - Na 139/ K 3.75/ Cl 101
  - CRP 325
  - LDH 422
  - Trp 24
  - Ddimers 574
  - IL-6 25 (N < 7)
  - Ferritine 103
  - ProBNP 13362

**2- Do you hospitalize her?**

**If yes, Ward or ICU?**

**3- What treatment will you prescribe for her?**

## Treatment:

Rocephine 2 gIV OD, Zinc, hydroxychloroquine, vit D & C, Azithromycine, Lovenox 60 mg BID, Lasix 1g IVSP & BIPAP with high flow oxygen

**4- How do you monitor her?**

## **Monitoring:**

Deterioration with excessive Oxygen need.

Intubation discussed with family & avoided with palliative care decision.

Persistent fever

Clinical deterioration with increased dyspnea & digestive hemorrhage

Deterioration of blood tests

**4- What is your plan now after 48h of  
monitoring?**

**Thank you for your  
participation**
